# Supplementary material for: ConsistentFeature: A Plug-and-Play Component for Neural Network Regularization
Source: arXiv:2412.01476 source file (2025-01-24)
Supplement: Supplementary file 1 [file _supplementary.tex]

\input{_constants}
\review % \review OR \cameraready

\documentclass[10pt,twocolumn,letterpaper]{article}
\input{cvpr_header}
\myexternaldocument{_main}
\begin{document}
% %% TITLE
\title{\paperTitle}
\author{\authorBlock}
\maketitlesupplementary
\appendix
\input{12_appendix}

% {\small
% \bibliographystyle{ieeenat_fullname}
% \bibliography{11_references}
% }

\end{document}
